# Supplementary material for: Euclid preparation: Determining the weak lensing mass accuracy and precision for galaxy clusters
Source: arXiv:2409.02783 source file (2024-12-18)
Supplement: Supplementary file 1 [file Configuration.tex]

% Configuration

\section{COMB-CL configuration} \label{COMB-CL configuration}

%----------------------------------------------------------------------------------------
